# Supplementary material for: Mimetic framework on curvilinear quadrilaterals of arbitrary order
Source: arXiv:1111.4304 source file (2011-11-18)
Supplement: Supplementary file 1 [file frameworkAppendix.tex]

\section{Tensor products}

%%%%%%%%%%%%%%%%%%%%%%%%%%%%%%%%%%%%%%%%%%%%%%%%%%%%%%%%%%%%%%%%%%%%%%%
\subsection{Tensor product of cell complexes}\label{algtoptensor}
%%%%%%%%%%%%%%%%%%%%%%%%%%%%%%%%%%%%%%%%%%%%%%%%%%%%%%%%%%%%%%%%%%%%%%%
This subsection is mainly based on Chapters XI and XIII of Massey, \cite{Massey1}.
In Section~\ref{sec:MSEM} of this paper we will discuss a spectral method which respects these structures from differential geometry/algebraic topology. This implementation makes use of tensor products which can also be introduced at the discrete level as is shown by the next definition:
\begin{definition}[\textbf{Tensor product of cell complexes}]\label{tensor_product_cell_complexes} \cite{Massey1}
Let $\bar{D}$ be a cell complex in the manifold $\manifold{M}$ with boundary operator $\bar{\partial}$ and $\hat{D}$ another cell complex in the manifold $\manifold{N}$ with boundary operator $\hat{\partial}$, then the {\em tensor product} $D = \bar{D} \otimes \hat{D}$ is the chain complex defined as follows: The $k$-cells are given by
\begin{equation}
C_k = \sum_{p+q=k} \bar{C}_p \otimes \hat{C}_q \;,
\end{equation}
and the homomorphism $\partial\,:\, C_k \rightarrow C_{k-1}$ is defined by
\begin{equation}
\partial \left ( \kchain{c}{p} \otimes \kchain{c}{q} \right ) = \left ( \bar{\partial} \kchain{c}{p} \right ) \otimes \kchain{c}{q} + (-1)^p \kchain{c}{p} \otimes \left ( \hat{\partial} \kchain{c}{q} \right ) \;,
\label{eq:boundary_on_tensor_prod_chains}
\end{equation}
for all $\kchain{c}{p} \in \bar{C}_p(\bar{D})$ and $\kchain{c}{q} \in \hat{C}_q(\tilde{D})$ with $p+q=k$.
\end{definition}
\begin{lemma}
$\partial \circ \partial \equiv 0$ in $D = \bar{D} \otimes \hat{D}$.
\end{lemma}
The proof follows directly from the definition of the tensor product and the fact that $\bar{\partial} \circ \bar{\partial} = \hat{\partial} \circ \hat{\partial} \equiv 0$. It can be shown \cite{Massey1} that the tensor product of non-degenerate $p$-cells in $\bar{D}$ and non-degenerate $q$-cells in $\tilde{D}$ yield non-degenerate $k$-cells in $D$.

\begin{theorem}\label{Commutation_tensor_chains} 
Let $\kchain{c}{p} \in C_p(\bar{D})$ and $\kchain{c}{q} \in C_q(\hat{D})$, then $\kchain{c}{p} \otimes \kchain{c}{q} \in C_p(\bar{D}) \otimes C_q(\hat{D})$ and we have that
\[ \kchain{c}{q} \otimes \kchain{c}{p} = (-1)^{pq} \kchain{c}{p} \otimes \kchain{c}{q} \;.\]
\end{theorem}
The proof of this theorem relies on the Eilenberg-Zilber theorem, \cite{Massey2}, which asserts that the chain complex of the product of two spaces, $C(\bar{D} \times \hat{D})$ is chain homotopic equivalent to the tensor product of the chain complexes in $\bar{D}$ and $\hat{D}$, i.e. $C(\bar{D}) \otimes C(\hat{D})$. The full proof of the Eilenberg-Zilber theorem is beyond the scope of this paper, but we briefly describe those ingredients which are essential for setting up higher order mimetic schemes.
\begin{proof}
For $0$-cells $\bar{\mathbf{c}}_{(0)} \in C_0(\bar{D})$ and $\hat{\mathbf{c}}_{(0)} \in C_0(\hat{D})$ it is straightforward to prove that $\bar{\mathbf{c}}_{(0)} \otimes \hat{\mathbf{c}}_{(0)} = \hat{\mathbf{c}}_{(0)} \otimes \bar{\mathbf{c}}_{(0)}$. Now assume that we know that this relation holds for all $\kchain{c}{(p-1)} \in C_{p-1}(\bar{D})$ and $\kchain{c}{q} \in C_q(\hat{D})$, and for all $\kchain{c}{p} \in C_p(\bar{D})$ and $\kchain{c}{(q-1)} \in C_{q-1}(\hat{D})$, then for $\kchain{c}{p} \in C_p(\bar{D})$ and $\kchain{c}{q} \in C_q(\hat{D})$, we have
\begin{eqnarray*}
\partial \left ( \kchain{c}{p} \otimes \kchain{c}{q} \right ) & \stackrel{(\ref{eq:boundary_on_tensor_prod_chains})}{=} & \left ( \bar{\partial} \kchain{c}{p} \right ) \otimes \kchain{c}{q} + (-1)^p \kchain{c}{p} \otimes \left ( \hat{\partial} \kchain{c}{q} \right ) \\
 & = & (-1)^{(p-1)q} \kchain{c}{q} \otimes \left ( \bar{\partial}\kchain{c}{p} \right ) + (-1)^{p+p(q-1)} \left ( \hat{\partial} \kchain{c}{q} \right ) \otimes \kchain{c}{p} \;\;\;\; \mbox{\tiny{(induction assumption)}} \\
 & = & (-1)^{pq} \left [ \left ( \hat{\partial} \kchain{c}{q} \right ) \otimes \kchain{c}{p} + (-1)^q \kchain{c}{q} \otimes \left ( \bar{\partial} \kchain{c}{p} \right )  \right ] \\
 & = & (-1)^{pq} \partial \left ( \kchain{c}{q} \otimes \kchain{c}{p} \right ) \;.
\end{eqnarray*}
Therefore, we have that
\begin{equation}
\kchain{c}{p} \otimes \kchain{c}{q} = (-1)^{pq} \kchain{c}{q} \otimes \kchain{c}{p} + \kchain{z}{p+q}\;,\;\;\; \forall \kchain{z}{p+q} \in Z_{p+q}(\bar{D}\times \hat{D})\;.
\label{homotopy_equivalence_tensor_product_chains}
\end{equation}
So, whatever the choice of boundary chain $\kchain{z}{p+q}$, all tensor products will be homologous. This proves the theorem.
\end{proof}

\begin{remark}
In Remark~\ref{maifold_independence_generalized_Stokes} following the definition of the generalized Stokes' Theorem, we observed that to the $(k+1)$-dimensional manifold ${\mathcal M}$ we can add a boundaryless, $(k+1)$-dimensional manifold $\bar{\mathcal M}$ with $\partial \bar{\mathcal M}=0$,  without affecting the generalized Stokes Theorem. The definition of the coboundary operator, Definition~\ref{def:coboundary_operator}, mimics the generalized Stokes Theorem in a topological setting. Also in this definition we could have added an arbitrary cycle chain $\kchain{z}{k+1} \in Z_{k+1}(D)$.
\[ \langle \dederiv \kcochain{c}{k}, \kchain{c}{k+1} + \kchain{z}{k+1} \rangle = \langle \kcochain{c}{k}, \partial \kchain{c}{k+1} + \partial \kchain{z}{k+1} \rangle = \langle \kcochain{c}{k}, \partial \kchain{c}{k+1}  \rangle = \langle \dederiv \kcochain{c}{k}, \kchain{c}{k+1} \rangle \;.\]
So, despite the fact the commutation relation for the tensor product of chains is unique modulo boundaries, we can write tensor products for $k$-chains without affecting the discrete analogue of Stokes' Theorem or the definition of the coboundary operator.
\end{remark}

\begin{remark}
In the relation $\kchain{c}{q} \otimes \kchain{c}{p} = (-1)^{pq} \kchain{c}{p} \otimes \kchain{c}{q}$, the factor $(-1)^{pq}$ accounts for a change in orientation. When $pq$ is even, the orientation remains the same, while for $pq$ is odd, the orientation changes sign. Therefore, the use of tensor products accounts for possible changes in orientation at the discrete level. The values $+1$ and $-1$ are represented in the incidence matrices.
\end{remark}

\begin{definition}[\textbf{Tensor product of cochains}]
Let $\kcochain{c}{p} \in C^p(\bar{D})$ and $\kcochain{c}{q} \in C^q(\hat{D})$, then $\kcochain{c}{p} \otimes \kcochain{c}{q} \in C^p(\bar{D}) \otimes C^q(\hat{D})$, where the action of the tensor product of cochains on the tensor product of chains is given by
\[ \langle \kcochain{c}{p} \otimes \kcochain{c}{q}, \kchain{c}{p} \otimes \kchain{c}{q} \rangle = \langle \kcochain{c}{p},\kchain{c}{p} \rangle_{\bar{D}} \cdot \langle \kcochain{c}{q},\kchain{c}{q} \rangle_{\hat{D}} \;.\]
\end{definition}

%Using the fact that the coboundary operator is the formal adjoint of the boundary operator and the action of the boundary operator on the tensor product of chains, (\ref{eq:boundary_on_tensor_prod_chains}), we have that
%\begin{equation}
%\delta \left ( \kcochain{c}{p} \otimes \kcochain{c}{q} \right ) = \left ( \delta \kcochain{c}{p} \right ) \otimes \kcochain{c}{q} + (-1)^p \kcochain{c}{p} \otimes \left ( \delta \kcochain{c}{q} \right ) \;.
%\end{equation}

\begin{lemma}\label{Commutation_cochain_tensor}
Let $\kcochain{c}{p} \in C^p(\bar{D})$ and $\kcochain{c}{q} \in C^q(\hat{D})$, then $\kcochain{c}{p} \otimes \kcochain{c}{q} \in C^{p+q}(\bar{D} \times \hat{D})$, then we have that
\[ \kcochain{c}{q} \otimes \kcochain{c}{p} = (-1)^{pq} \kcochain{c}{p} \otimes \kcochain{c}{q} \;. \]
\end{lemma}
\begin{proof}
Using Theorem~\ref{Commutation_tensor_chains} we have
\begin{eqnarray*}
\langle \kcochain{c}{q} \otimes \kcochain{c}{p}, \kchain{c}{p} \otimes \kchain{c}{q}  \rangle & := & \langle \kcochain{c}{q} \otimes \kcochain{c}{p}, (-1)^{pq}\kchain{c}{q} \otimes \kchain{c}{p}  \rangle \\
 & = & (-1)^{pq} \langle \kcochain{c}{p},\kchain{c}{p} \rangle \cdot \langle \kcochain{c}{q},\kchain{c}{q} \rangle \\
 & = & (-1)^{pq} \langle \kcochain{c}{p} \otimes \kcochain{c}{q}, \kchain{c}{p} \otimes \kchain{c}{q}  \rangle.
 \end{eqnarray*}
 This holds for all $\kchain{c}{p} \in C_p(\bar{D})$ and $\kchain{c}{q} \in C_q(\hat{D})$ and therefore
\[ \kcochain{c}{p} \otimes \kcochain{c}{q} = (-1)^{pq}\kcochain{c}{q} \otimes \kcochain{c}{p} \;.\]
\end{proof}

\begin{remark}
This relation shows that the tensor product of cochains mimics relation (\ref{wedge::skew_symmetry}) of the wedge product. It is straightforward to show that the tensor product of cochains satisfies {\em all} properties of the wedge product (2.2a-2.2d). Note, however, that the converse is {\em not} true, i.e. the wedge product is not fully described in terms of cochains. As long as the cochain spaces are defined over different cell complexes, i.e. $C^p(\bar{D})$ and $C^q(\hat{D})$, for $\bar{D} \neq \hat{D}$, then there is a one-to-one correspondence between the tensor product of cochains and the wedge product of differential forms. But if $\bar{D}=\hat{D}$, which is for instance the case in a wedge product of the form $a(x) \wedge b(x)\,\ederiv x$, the one-to-one connection between the tensor product of cochains and wedge product of differential forms breaks down. 
%A possible means to define such a product in algebaric topology is the {\em cup product}, but the cup product is only distributive for closed differential forms. 
Therefore, in Section~\ref{mimeticoperators}, a discrete wedge product will be defined which approximates the continuous wedge product.
\end{remark}

\begin{definition}
An expression of the form $\left \langle \kcochain{c}{k}, \kchain{c}{l} \right \rangle$ for $k \neq l$ is not defined and whenever such an expression occurs, we set
\begin{equation}
\left \langle \kcochain{c}{k}, \kchain{c}{l} \right \rangle := 0\;,\;\;\; k \neq l\;.
\label{cochain_k_chain_l_undefined}
\end{equation}
\end{definition}

\begin{lemma}\label{lemma:discrete_Leibniz_rule}
Let $\bar{D}$ be a cell complex in the manifold $\manifold{M}$ with coboundary operator $\bar{\delta}$ and let $\hat{D}$ be another cell complex over the manifold $\manifold{N}$ with coboundary operator $\hat{\delta}$, then the coboundary operator $\delta$ of of the tensor product of $\kcochain{c}{p} \in C^p(\bar{D})$ and $\kcochain{c}{q} \in C^q(\hat{D})$ is given by
\[ \delta \left ( \kcochain{c}{p} \otimes \kcochain{c}{q} \right ) =  \left ( \bar{\delta} \kcochain{c}{p} \right ) \otimes \kcochain{c}{q} + \left (-1 \right )^p \kcochain{c}{p} \otimes \left ( \hat{\delta} \kcochain{c}{q} \right ) \;.\]
\end{lemma}

\begin{proof}
Using the generalized Stokes Theorem repeatedly, we have for all $\kchain{c}{p+1} \in C_{p+1}(\bar{D})$ and $\kchain{c}{q} \in C_q(\hat{D})$ and all $\kchain{c}{p} \in C_{p}(\bar{D})$ and $\kchain{c}{q+1} \in C_{q+1}(\hat{D})$
\begin{align*}
\left \langle \delta \left ( \kcochain{c}{p} \right. \right . & \left . \left . \otimes  \kcochain{c}{q}   \right ) , \kchain{c}{p+1} \otimes \kchain{c}{q} + \kchain{c}{p} \otimes \kchain{c}{q+1} \right \rangle  =  \left \langle  \kcochain{c}{p} \otimes \kcochain{c}{q} , \partial \left ( \kchain{c}{p+1} \otimes \kchain{c}{q} + \kchain{c}{p} \otimes \kchain{c}{q+1}\right ) \right \rangle \\
 & =  \left \langle  \kcochain{c}{p} \otimes \kcochain{c}{q} , \left ( \bar{\partial} \kchain{c}{p+1} \right ) \otimes \kchain{c}{q} + \left ( \bar{\partial} \kchain{c}{p} \right ) \otimes \kchain{c}{q+1}\right \rangle + \\
 & \quad    \left \langle  \kcochain{c}{p} \otimes \kcochain{c}{q} , (-1)^{p+1}  \kchain{c}{p+1} \otimes \left ( \hat{\partial} \kchain{c}{q} \right ) + (-1)^{p}  \kchain{c}{p} \otimes \left ( \hat{\partial} \kchain{c}{q+1} \right ) \right \rangle \\
 & \stackrel{(\ref{cochain_k_chain_l_undefined})}{=}  \left \langle  \kcochain{c}{p} \otimes \kcochain{c}{q} , \left ( \bar{\partial} \kchain{c}{p+1} \right ) \otimes \kchain{c}{q} + (-1)^p \kchain{c}{p} \otimes \left ( \hat{\partial} \kchain{c}{q+1} \right ) \right \rangle  \\
 &  =  \left \langle  \kcochain{c}{p}, \bar{\partial}\kchain{c}{p+1} \right \rangle \cdot \left \langle \kcochain{c}{q} , \kchain{c}{q} \right \rangle + (-1)^p \left \langle  \kcochain{c}{p}, \kchain{c}{p} \right \rangle \cdot \left \langle \kcochain{c}{q}, \hat{\partial} \kchain{c}{q+1} \right \rangle \\
 &  =  \left \langle \bar{\delta} \kcochain{c}{p}, \kchain{c}{p+1} \right \rangle \cdot \left \langle \kcochain{c}{q} , \kchain{c}{q} \right \rangle + (-1)^p \left \langle  \kcochain{c}{p}, \kchain{c}{p} \right \rangle \cdot \left \langle \hat{\delta}\kcochain{c}{q}, \kchain{c}{q+1} \right \rangle \\
 & =  \left \langle \bar{\delta} \kcochain{c}{p} \otimes \kcochain{c}{q},\kchain{c}{p+1} \otimes \kchain{c}{q} \right \rangle + (-1)^p \left \langle \kcochain{c}{p} \otimes \hat{\delta} \kcochain{c}{q}, \kchain{c}{p} \otimes \kchain{c}{q+1} \right \rangle \\
 & \stackrel{(\ref{cochain_k_chain_l_undefined})}{=} \left \langle \bar{\delta} \kcochain{c}{p} \otimes \kcochain{c}{q} + (-1)^p \kcochain{c}{p} \otimes \hat{\delta} \kcochain{c}{q}, \kchain{c}{p+1} \otimes \kchain{c}{q} + \kchain{c}{p} \otimes \kchain{c}{q+1} \right \rangle \;,
\end{align*}
where in the last line we add $(p+q+1)$-chains, which due to (\ref{cochain_k_chain_l_undefined}) do not contribute.
\end{proof}

\begin{remark}
We already noted that the tensor product between different cell complexes behaves in a similar way as the wedge product. Lemma~\ref{lemma:discrete_Leibniz_rule} shows that the coboundary operator applied to a tensor product of cochains behaves in the same way as the exterior derivative applied to the wedge product of differential forms, as given in (\ref{eq::dif_and_wedge}) of Definition~\ref{def:exterior_derivative}.
\end{remark}

\begin{remark}
A general $(p+q+1)$-chain in terms of tensor products of $\bar{D}$ and $\hat{D}$ is of the form
\[ \kchain{c}{p+q+1} = \sum_{k=0}^{p+q+1} \kchain{c}{k} \otimes \kchain{c}{p+q-k+1}\;,\;\;\; \kchain{c}{k} \in C_k(\bar{D})\mbox{ and } \kchain{c}{p+q-k+1} \in C_{p+q-k+1}(\hat{D})\;.\]
In the proof only the non-zero contributions in this summation are retained.
\end{remark}

\subsection{Tensor products}\label{mimoptensor}
Any singular $k$-cube was considered to be a map $\tau_{(k)}\,:\,I^k \rightarrow X$, see \defref{def:kcube}. Now we are going to consider tensor product of one dimensional singular $k$-cubes, with $k=d(i)$ for all coordinate directions $1\leq i\leq n$,
\[ \bigotimes_{i=1}^n \tau_{d(i)}(I^{d(i)}) :=\tau_{d(1)}(I^{d(1)}) \otimes \tau_{(d(2))}(I^{d(2)}) \otimes \dots \otimes \tau_{d(n)}(I^{d(n)}) \,\longrightarrow \, X \;,\] 
in which $\tau_{d(i)}$ is a one-dimensional $0$-cell if $d(i)=0$ and a one-dimensional $1$cell if $d(i)=1$, such that the number of $1$-cells in this tensor product is equal to $k$, i.e. $\sum_{i=1}^n d(i) = k$.

\begin{definition}[\textbf{Tensor reduction operator}]\label{def:tensorreduction}
Define the reduction operator $\reduction^\otimes\, : \,\kformspacedomain{k}{\Omega \subset \mathbb{R}^n} \rightarrow \bigotimes_{i=1}^n C^{d(i)}$ as the tensor product of $n$ one-dimensional reduction operators over the cells $\tau_{d(i)}$,
\begin{equation}
\left\langle \reduction^\otimes \kdifform{a}{k} , \bigotimes_{i=1}^n \tau_{d(i),i} \right\rangle := \left\langle \bigotimes_{j=1}^n \reduction_j \kdifform{a}{k},\bigotimes_{i=1}^n \tau_{d(i)} \right\rangle =  \int_{\tau_{d(1)}} \dots \int_{\tau{d(n)}} \kdifform{a}{k}.
\end{equation}
Essentially, the reduction operator is decomposed into integrals in each coordinate direction using Fubini's Theorem, \cite{spivak1998calculus}.
\end{definition}
\begin{example}
Let $n=3$ and $\kdifform{a}{2}=dx \wedge dy$. Let the tensor $2$-chain be given by $\kchain{c}{2} =[-1,1]\otimes [0,1] \otimes \{5\}$, then
\[ \langle R^\otimes \kdifform{a}{k}, \kchain{c}{2} \rangle = \left . \int_{-1}^1 \int_{0}^1 \, dxdy \right |_{z=5} = 2\;.\]
for the reduction of the $2$-form $\kdifform{b}{2} = dy \wedge dx$, we either need to write the differential form in the '$x$-$y$-$z$'-sequence, i.e. $\kdifform{b}{2} = - dx \wedge dy$, or write the $2$-chain in the '$y$-$x$-$z$'-sequence using $\kchain{c}{1}(x) \otimes \kchain{c}{1}(y)\otimes \kchain{c}{0}(z) = - \kchain{c}{1}(y) \otimes \kchain{c}{1}(x)\otimes \kchain{c}{0}(z)$, Theorem~\ref{Commutation_tensor_chains}, which in both cases yields
\[ \langle R^\otimes \kdifform{b}{k}, \kchain{c}{2} \rangle = - 2\;.\]
This example shows that $\reduction^\otimes \left ( dy \wedge dx \right ) = - \reduction^\otimes \left ( dx \wedge dy \right )$. So if the orientation of the geometry changes sign, then also the associated cochain changes sign. This is one of the basic physical properties that was mentioned in the introduction.
\end{example}

In order to show that $\reduction^\otimes$ is indeed a reduction operator, we need to establish that $\reduction^\otimes \ederiv = \delta \reduction^\otimes$. 
\begin{lemma}
The tensor reduction operator $\reduction^\otimes$ satisfies $\reduction^\otimes \ederiv = \delta \reduction^\otimes$. 
\end{lemma}
\begin{proof}
Let $\kchain{c}{k+1} = \tau_{d(1)} \otimes \ldots \otimes \tau_{d(n)}$ with $\sum_{i=1}^n d(i) = k+1$, then

\begin{gather*}
\left \langle \delta \reduction^\otimes \kdifform{a}{k},\kchain{c}{k+1}\right \rangle  \stackrel{\eqref{eq::algTop_codifferential_dual}}{=} \left \langle  \reduction^\otimes \kdifform{a}{k},\partial \kchain{c}{k+1}\right \rangle \\
  \stackrel{\eqref{eq:boundary_on_tensor_prod_chains}}{=}\int_{\partial \tau_{d(1)}}\int_{\tau_{d(2)}}\hdots \int_{\tau_{d(n)}} \kdifform{a}{k} + \hdots + (-1)^{\sum_{k=1}^{i-1} d(k)} \int_{\tau_{d(1)}} \hdots \int_{\partial \tau_{d(i)}} \hdots \int_{\tau_{d(n),n}} \kdifform{a}{k} \\
+ \hdots + (-1)^{\sum_{k=1}^{n-1} d(k)} \int_{\tau_{d(1)}} \ldots \int_{\partial \tau_{d(n)}} \kdifform{a}{k}\\
  \stackrel{\eqref{eq::difGeom_stokes_theorem}}{=} \int_{\tau_{d(1)}} \int_{\tau_{d(2)}}\ldots \int_{\tau_{d(n)}} \frac{\partial}{\partial x^1} \kdifform{a}{k} \wedge dx^1  + \hdots + (-1)^{\sum_{k=1}^{i-1} d(k)} \int_{\tau_{d(1)}} \ldots \int_{\tau_{d(i)}} \ldots \int_{\tau_{d(n)}} \frac{\partial}{\partial x^i}\kdifform{a}{k} \wedge dx^i \\
+ \hdots + (-1)^{\sum_{k=1}^{n-1} d(k)} \int_{\tau_{d(1)}} \hdots \int_{\tau_{d(n)}} \frac{\partial}{\partial x^n} \kdifform{a}{k} \wedge dx^n\\
  =\left \langle \reduction^\otimes \ederiv \kdifform{a}{k}, \kchain{c}{k+1} \right \rangle.
\end{gather*}
Note that whenever $d(i)=0$, $\partial \tau_{d(i),i} = \emptyset$ and the entire iterated integral cancels from the summation. In this case $\partial/\partial x^i \kdifform{a}{k} \wedge dx^i$ cannot be intgerated over $\tau_{d(i),i}$ and also this whole iterated integral needs to be set to zero. This is analogous to (\ref{cochain_k_chain_l_undefined}).
\end{proof}

\begin{remark}
The appearance of the factors $(-1)^{\sum_{k=1}^{i-1} d(k)}$ either produce a $1$ or $-1$. These factors are determined by the topology of the cell complex and the orientation chosen in the cell-complex and are contained in the incidence matrix. Whenever an iterated integral does not contribute to the summation, this is indicated in the incidence matrix by a $0$ entry. 
\end{remark}

Furthermore, we need to show that $\reduction^\otimes \Phi^\star = \Phi^\sharp \reduction^\otimes$.
\begin{lemma}
Let $\Phi\,:\,\mathbb{R}^n \longrightarrow \mathbb{R}^n$ be a continuous tensor map of the form $\Phi(x^1, \ldots, x^n) = \Phi_1(x^1) \cdot \ldots \cdot \Phi_n(x^n)$, then $\Phi^\sharp \reduction^\otimes = \reduction^\otimes \Phi^\star$.
\end{lemma}

Before, we can prove this, we need to show that the associated chain map commutes with the boundary operator, i.e.
\begin{equation}
\Phi_\sharp \left ( \kchain{c}{d(1)} \otimes \ldots \otimes \kchain{c}{d(n)} \right ) = \left ( \Phi_{\sharp,1} \kchain{c}{d(1)} \right ) \otimes \ldots \otimes \left ( \Phi_{\sharp,n} \kchain{c}{d(n)} \right ) \;.
\label{tensor_chain_map}
\end{equation}
This is the case, because
\begin{gather*}
\partial \Phi_\sharp \left ( \kchain{c}{d(1)} \otimes \ldots \otimes \kchain{c}{d(n)} \right ) = \partial \left [ \left ( \Phi_{\sharp,1} \kchain{c}{d(1)} \right ) \otimes \ldots \otimes \left ( \Phi_{\sharp,n} \kchain{c}{d(n)} \right ) \right ] \\
 \stackrel{\mathrm{Lem}\;\ref{lemma:discrete_Leibniz_rule}}{=}  \left ( \partial \Phi_{\sharp,1} \kchain{c}{d(1)} \right ) \otimes \ldots \otimes \left ( \Phi_{\sharp,n} \kchain{c}{d(n)} \right ) + \hdots + (-1)^{\sum_{k=1}^{i-1}d(k)}  \left ( \Phi_{\sharp,1} \kchain{c}{d(1)} \right ) \otimes \ldots \left ( \partial \Phi_{\sharp,i} \kchain{c}{d(i)} \right ) \ldots \otimes \left ( \Phi_{\sharp,n} \kchain{c}{d(n)} \right )\\
  + \hdots + (-1)^{\sum_{k=1}^{n-1}d(k)}  \left ( \Phi_{\sharp,1} \kchain{c}{d(1)} \right ) \otimes \ldots \otimes \left ( \partial \Phi_{\sharp,n} \kchain{c}{d(n)} \right ) \\
 = \left (  \Phi_{\sharp,1} \partial \kchain{c}{d(1)} \right ) \otimes \ldots \otimes \left ( \Phi_{\sharp,n} \kchain{c}{d(n)} \right ) + \hdots +  (-1)^{\sum_{k=1}^{i-1}d(k)}  \left ( \Phi_{\sharp,1} \kchain{c}{d(1)} \right ) \otimes \ldots \left (  \Phi_{\sharp,i} \partial \kchain{c}{d(i)} \right ) \ldots \otimes \left ( \Phi_{\sharp,n} \kchain{c}{d(n)} \right ) \\
   + \hdots + (-1)^{\sum_{k=1}^{n-1}d(k)}  \left ( \Phi_{\sharp,1} \kchain{c}{d(1)} \right ) \otimes \ldots \otimes \left ( \Phi_{\sharp,n} \partial \kchain{c}{d(n)} \right ) \\
 \stackrel{\mathrm{Lem}\;\ref{lemma:discrete_Leibniz_rule}}{=} \Phi_\sharp \partial \left ( \kchain{c}{d(1)} \otimes \ldots \otimes \kchain{c}{d(n)} \right )
\end{gather*}

\begin{proof}
Let $\Phi$ be the continuous tensor map as given above. This maps induces a tensor chain map which commutes with the boundary operator and therefore leaves the topology of the cell complex unchanged. Then we have
\begin{gather*}
\left \langle \Phi^\sharp \reduction^\otimes \kdifform{a}{k}, \kchain{c}{d(1)}\otimes \ldots \otimes \kchain{c}{d(n)} \right \rangle = \left \langle \reduction^\otimes \kdifform{a}{k}, \left ( \Phi_{\sharp,1} \kchain{c}{d(1)} \right ) \otimes \ldots \otimes \left ( \Phi_{\sharp,n} \kchain{c}{d(n)} \right ) \right \rangle \\
 = \int_{\Phi_{\sharp,1} \kchain{c}{d(1)}} \dots \int_{\Phi_{\sharp,n} \kchain{c}{d(n)}} \kdifform{a}{k} 
 = \int_{\kchain{c}{d(1)}} \ldots \int_{\kchain{c}{d(n)}} \Phi_n^\star \ldots \Phi_1^\star \kdifform{a}{k} \\
 = \left \langle \reduction^\otimes  \Phi^\star \kdifform{a}{k}, \kchain{c}{d(1)}\otimes \ldots \otimes \kchain{c}{d(n)} \right \rangle.
\end{gather*}
\end{proof}
